# Supplementary material for: Linking the connectome to action: Emergent dynamics in a robotic model of C. elegans
Source: arXiv:2011.09057 source file (2020-11-18)
Supplement: Supplementary file 1 [file Gleiser_Supplementary.pdf]

# Linking the connectome to action: Emergent dynamics in a robotic model of C. elegans

# Supplementary material

Carlos E. Valencia Urbina[1,2,+], Sergio A. Cannas[3,+], and Pablo M. Gleiser[1,4,+,*]

**1** Medical Physics Department, Centro Atómico Bariloche, Río Negro 8400, Argentina.
**2** Instituto Balseiro, Universidad Nacional de Cuyo, Río Negro 8400, Argentina.
**3** Instituto de Física Enrique Gaviola (IFEG), Facultad de Matemática, Astronomía, Física y Computación, Universidad Nacional de Córdoba, Ciudad Universitaria, (5000), Córdoba, Argentina.
**4** Universidad Nacional de Río Negro, Bariloche, Río Negro 8400, Argentina.

*gleiser@cab.cnea.gov.ar

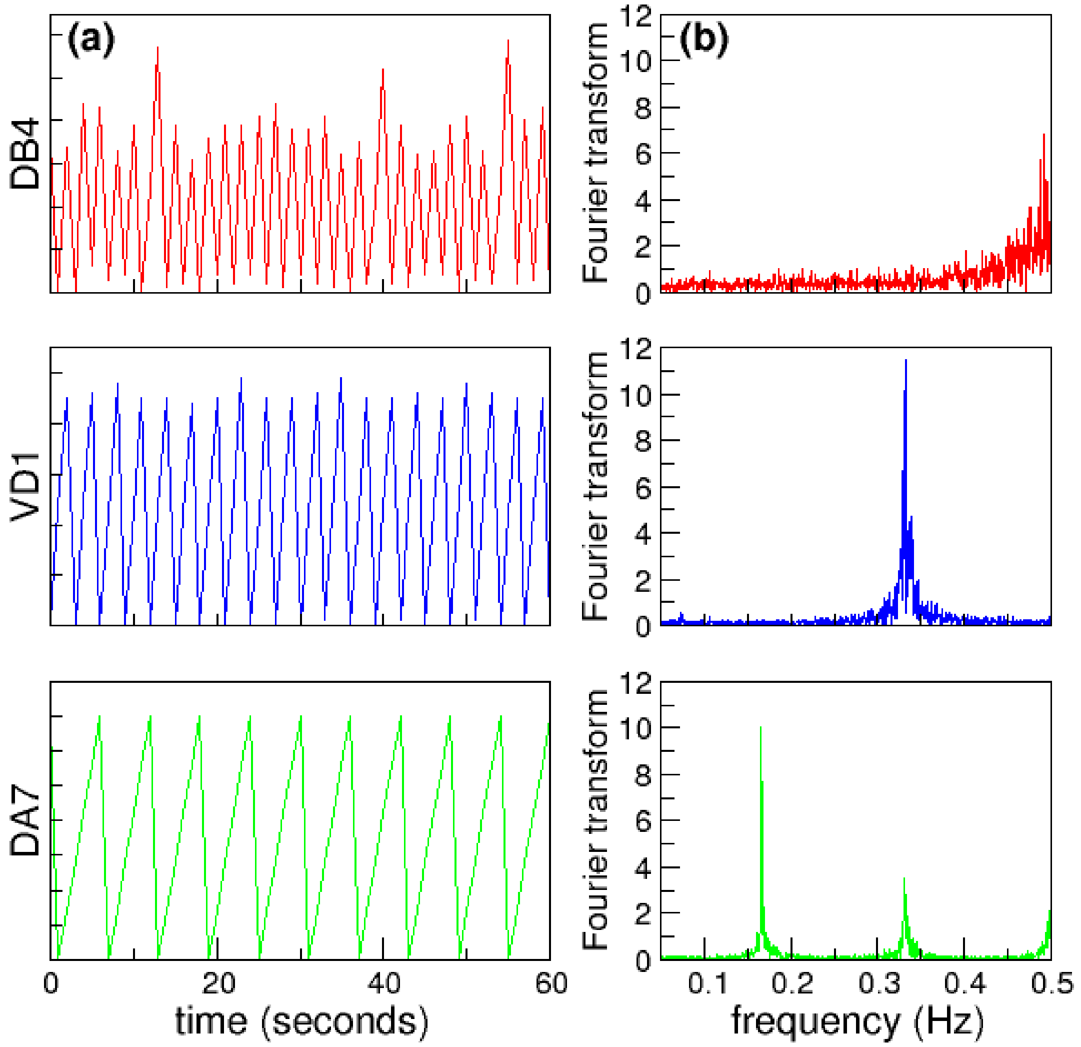


**Supplementary Figure S1**. **(a)** The signals of DA7 (green), VD1 (blue) and DB4 (red) in a 60 second time interval. **(b)** Fourier Transforms of the neurons presented in **(a)**, for a 20 minute long experiment.

| Neuron | Description | Ω | PC1 |
|---|---|---|---|
| DA7 | VCMN | 0.166 ± 0.001 | 2.7 ± 0.1 |
| AVL | RVCI | 0.164 ± 0.001 | 1.6 ± 0.1 |
| AS2 | VCMN | 0.163 ± 0.001 | 0.1 ± 0.1 |
| DB4 | VCMN | 0.165 ± 0.001 | 0.1 ± 0.1 |
| RMDL | VCMN | 0.167 ± 0.001 | -0.2 ± 0.1 |
| VA7 | VCMN | 0.166 ± 0.001 | -0.8 ± 0.1 |
| DD6 | VCMN | 0.166 ± 0.001 | -1.2 ± 0.1 |
| SABVR | RI | 0.162 ± 0.001 | -4.2 ± 0.1 |
| RID | RI | 0.164 ± 0.001 | -7.1 ± 0.1 |
| VD7 | VCMN | 0.165 ± 0.001 | -13.5 ± 0.1 |

**Supplementary Table S1A**. The table presents the neurons in synchronized cluster $\Omega_1$ , their description and corresponding characteristic frequency and first principal component weight PC1.

VCMN = Ventral Cord Motor Neuron, RVCI = Ring and Ventral Cord Interneuron, RI = Ring Interneuron.

| Neuron | Description | Ω | PC1 |
|---|---|---|---|
| VA11 | VCMN | 0.331 ± 0.001 | 15.3 ± 0.1 |
| VA6 | VCMN | 0.331 ± 0.001 | 9.8 ± 0.1 |
| DA5 | VCMN | 0.333 ± 0.001 | 7.4 ± 0.1 |
| VD3 | VCMN | 0.328 ± 0.001 | 3.9 ± 0.1 |
| VD1 | VCMN | 0.330 ± 0.001 | 0.6 ± 0.1 |
| DA1 | VCMN | 0.332 ± 0.001 | -1.7 ± 0.1 |
| AS11 | VCMN | 0.328 ± 0.001 | -2.5 ± 0.1 |
| DD3 | VCMN | 0.331 ± 0.001 | -6.4 ± 0.1 |
| VD4 | VCMN | 0.328 ± 0.001 | -7.1 ± 0.1 |
| VD6 | VCMN | 0.332 ± 0.001 | -12.7 ± 0.1 |

**Supplementary Table S1B**. The table presents the neurons in synchronized cluster $\Omega_2$ , their description and corresponding characteristic frequency and first principal component weight PC1.

VCMN = Ventral Cord Motor Neuron.

| Neuron | Description | Ω | PC1 |
|---|---|---|---|
| VA8 | VCMN | 0.498 ± 0.001 | 110.1 ± 0.1 |
| DA6 | VCMN | 0.496 ± 0.001 | 95.8 ± 0.1 |
| AVDL | VCI | 0.496 ± 0.001 | 76.1 ± 0.1 |
| AS7 | VCMN | 0.495 ± 0.001 | 29.9 ± 0.1 |
| AS8 | VCMN | 0.496 ± 0.001 | 17.8 ± 0.1 |
| AS9 | VCMN | 0.491 ± 0.001 | 5.7 ± 0.1 |
| PVCR | VCI | 0.488 ± 0.001 | 15.1 ± 0.1 |
| AVBL | VCI | 0.499 ± 0.001 | -10.1 ± 0.1 |
| DD4 | VCMN | 0.499 ± 0.001 | -51.2 ± 0.1 |
| AVAR | VCI | 0.489 ± 0.001 | -84.9 ± 0.1 |
| AVAL | VCI | 0.499 ± 0.001 | -99.8 ± 0.1 |

**Supplementary Table S1C**. The table presents the neurons in synchronized cluster $\Omega_3$ , their description and corresponding characteristic frequency and first principal component weight PC1.

VCMN = Ventral Cord Motor Neuron, VCI = Ventral Cord Interneuron.

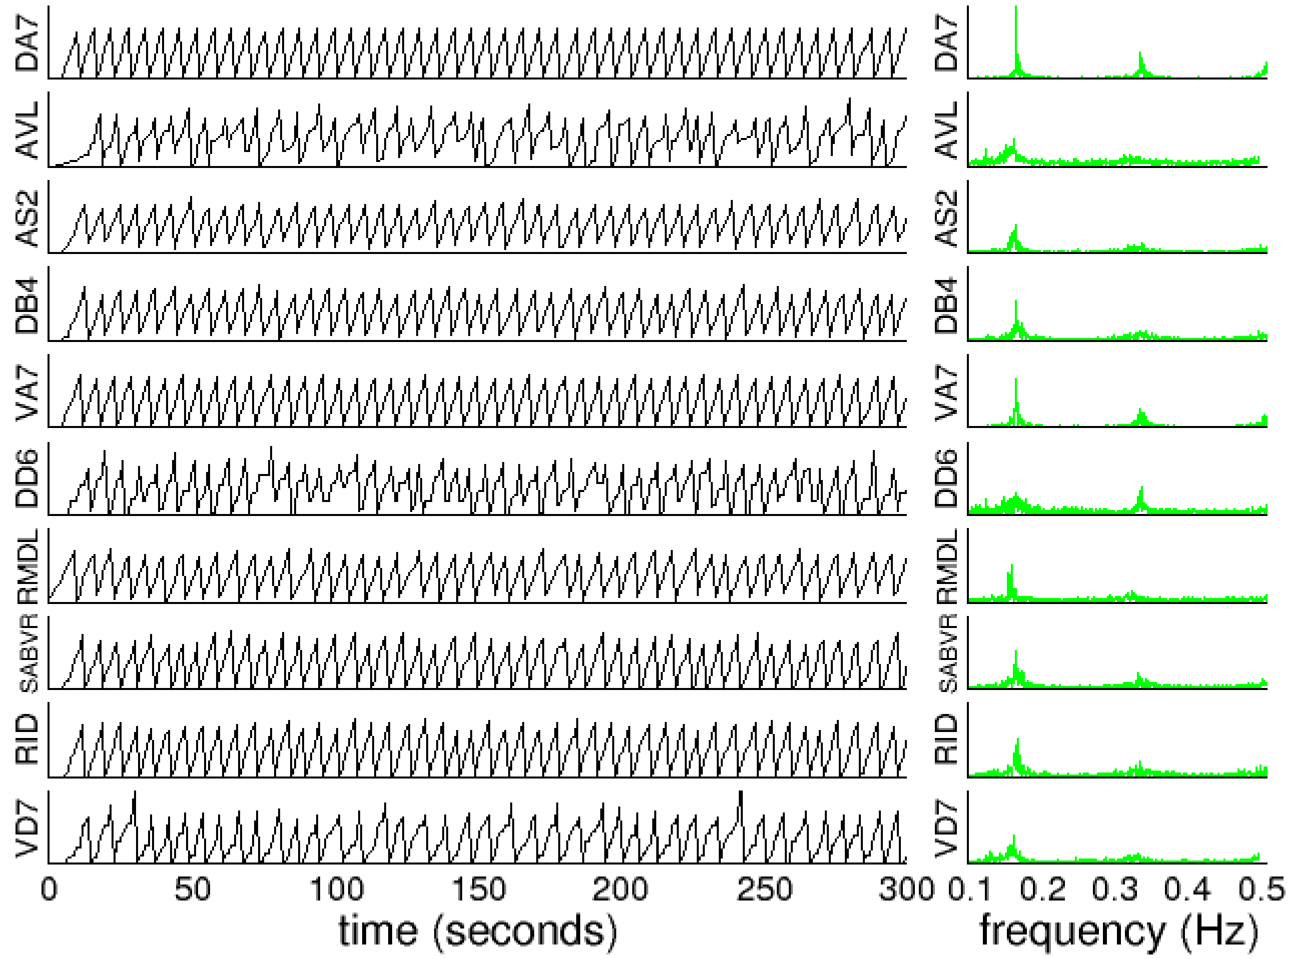


**Supplementary Figure S2A**. The signals of all the neurons in the synchronized cluster $\Omega_1$ in a five minute time interval, and their corresponding Fourier transforms in a 20 minute long experiment.

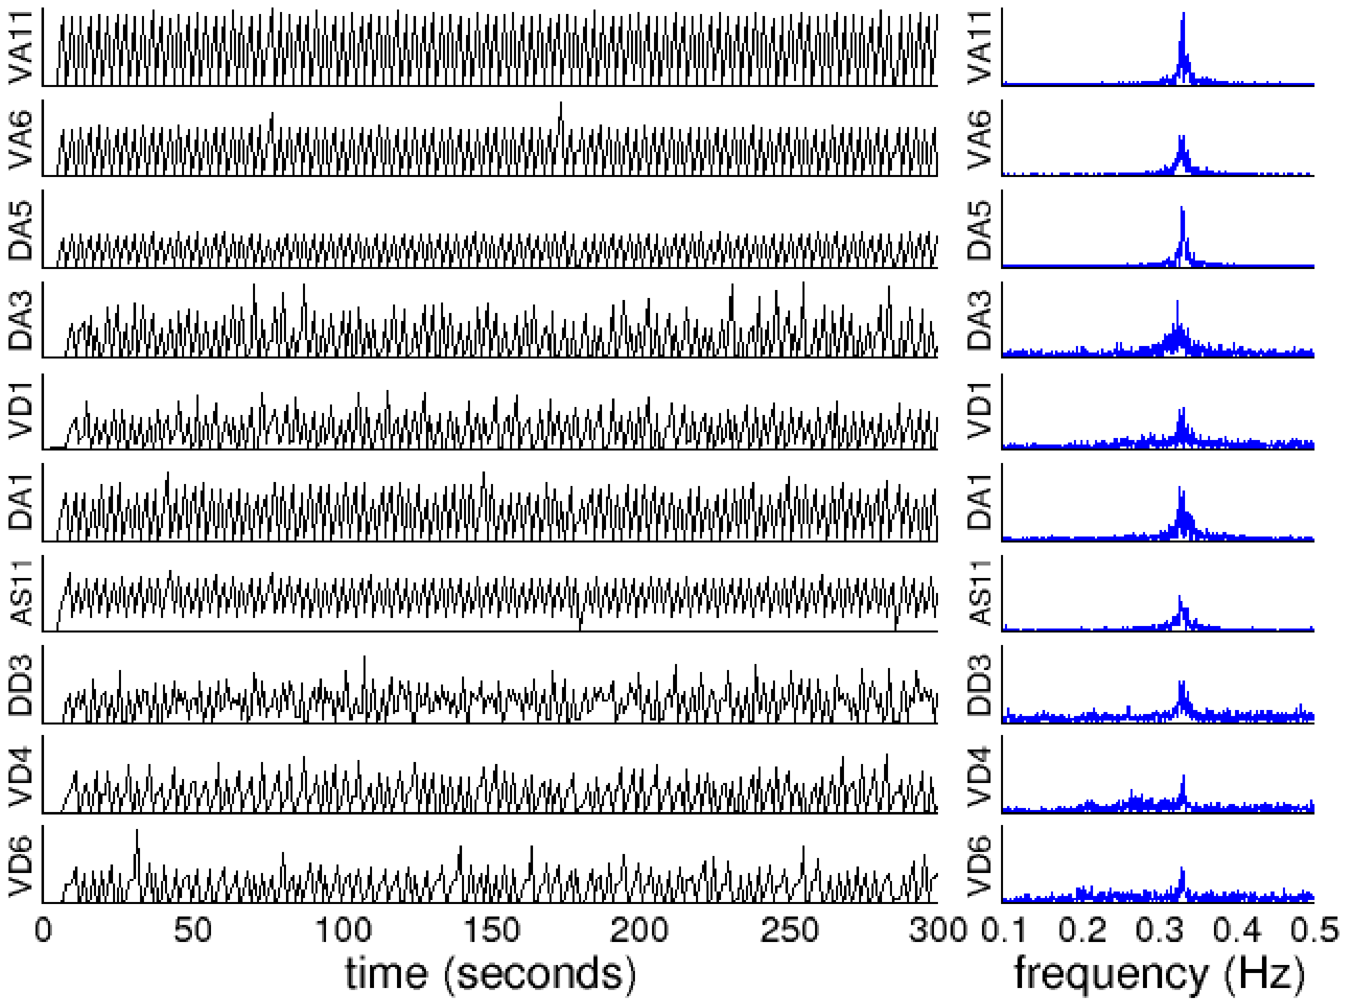


**Supplementary Figure S2B**. The signals of all the neurons in the synchronized cluster $\Omega_2$ in a five minute time interval, and their corresponding Fourier transforms in a 20 minute long experiment.

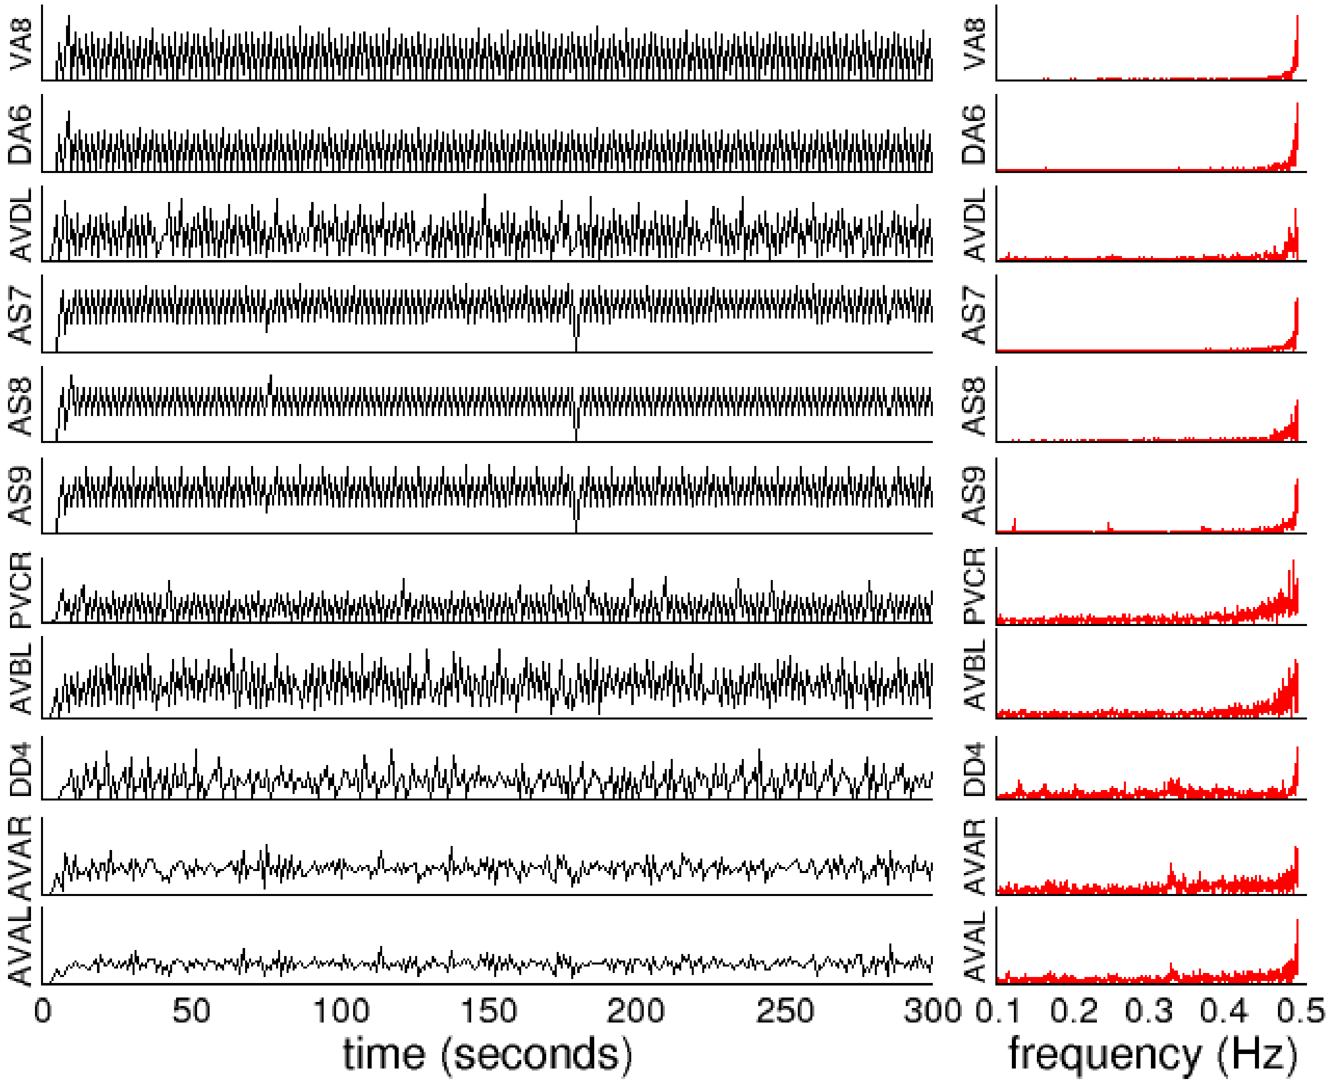


**Supplementary Figure S2C**. The signals of all the neurons in the synchronized cluster $\Omega_3$ in a five minute time interval, and their corresponding Fourier transforms in a 20 minute long experiment.

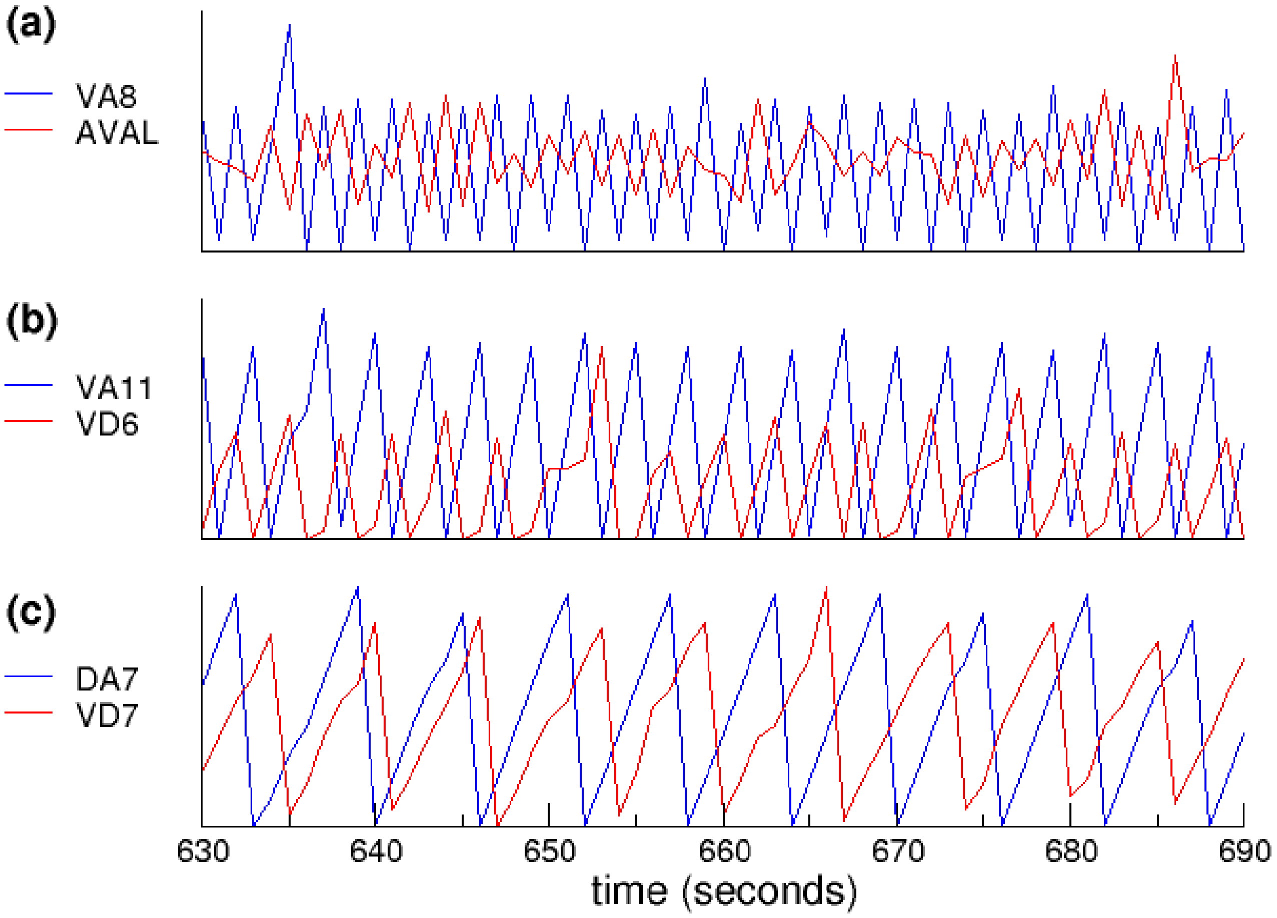


**Supplementary Figure S3**. Antiphase oscillations of neurons with the largest positive PC1 (blue) and lowest negative PC1 (red). (a) VA8 and AVAL in cluster $\Omega_3$, (b) VA11 and VD6 in cluster $\Omega_2$, and (c) DA7 and VD7 in cluster $\Omega_1$.

All figures are presented in the same 60 second time interval.

| Neuron | Forward | Backward |
|---|---|---|
| DA7 | 0.79 | 0.20 |
| VD7 | 0.48 | 0.50 |
| VA11 | 0.80 | 0.17 |
| VD6 | 0.50 | 0.46 |
| VA8 | 0.85 | 0.12 |
| AVAL | 0.59 | 0.39 |

**Supplementary Table S2**. Fraction of forward and backward events registered when the corresponding neurons fired. The fraction of events for the full 20 minute experiment was Forward = 0.69 and Backward = 0.28.
